# Supplementary material for: Poissonian communications: free space optical data transfer at the few-photon level
Source: arXiv:1801.07994 ancillary file (2018-01-24)
Supplement: Supplementary file 1 [file SinglePhoton_SupplementaryMaterial.pdf]

# Poissonian communications: optical wireless data transfer at the few-photon level: supplementary material

Alexander D. Griffiths<sup>1</sup>, Johannes Herrnsdorf<sup>1</sup>, Christopher Lowe<sup>2</sup>, Malcolm Macdonald<sup>2</sup>, Robert Henderson<sup>3</sup>, Michael J. Strain<sup>1,\*</sup>, and Martin D. Dawson<sup>1</sup>

<sup>1</sup>Institute of Photonics, University of Strathclyde, Glasgow

<sup>2</sup>Department of Mechanical & Aerospace Engineering, University of Strathclyde, Glasgow

<sup>3</sup>CMOS Sensors & Systems Group, University of Edinburgh, Edinburgh

\*Corresponding author: michael.strain@strath.ac.uk

January 23, 2018

## Abstract

This document provides supplementary information to Ultra-low light level communications using LED emitters. The document details the mathematical backing for a transmission scheme for optical wireless communications. The response of a single photon avalanche diode to input photon distributions is analysed, and transmission protocols developed. Furthermore, a method for synchronisation of transmitter and receiver is introduced, and simulations assess synchronisation performance. Symbol-level and frame-level synchronisation can be obtained, allowing real-time data transmission. Finally, the numerical method used to calculate received power from photon count rate is described.

## 1 Single photon detectors

Single-Photon Avalanche Diodes (SPADs) are different from other types of photo-diodes in that they do not give an analogue output signal as a response of optical input. They instead give discrete logic pulses that are triggered by single photons or other (undesired) discrete events. The exact timing of one such pulse cannot be predicted, but the probability  $P(t, t + \Delta t)$  that a pulse occurs in the time interval  $[t, t + \Delta t]$  can in principle be calculated:

$$P(t, t + \Delta t) = \int_t^{t+\Delta t} dt f(t) \quad (1)$$

Where  $f(t)$  is the temporal probability distribution of pulses. This means that with a single SPAD as detector, we cannot trigger directly from an optical waveform as we can with other types of photodiodes. There are two ways to deal with this:

1. Combine a number of SPADs to generate an output signal that can be triggered from.

2. Change the transmission protocol to eliminate the necessity for triggering.

Of course, the two approaches can also be combined. Here we examine the second approach. The achievable data rates are expected to be low, and the promise in the new scheme lies in potentially unrivalled dynamic range and ability to cope with low light levels and poor signal to noise ratio (SNR). The logic nature of the SPAD output and the statistical nature of the decoding process allow, efficient and relatively simple logic circuits, such as can be implemented in an ASIC, to decode the received data.

## 2 Master Equation

While the SPAD is in Geiger-mode, pulses are triggered by incident photons with a photon detection probability (PDP)  $\eta_{\text{PDP}}$  and also spontaneously triggered at a dark count rate  $R_{\text{dark}}$ :

$$f_{\text{Geiger}}(t) = \eta_{\text{PDP}}\rho_{ph}(t) + R_{\text{dark}} \quad (2)$$

Where  $\rho_{ph}(t)$  is the stream of incident photons. Once, a pulse is triggered, the SPAD goes through a recovery cycle, or dead time, of duration  $\tau_{\text{reset}}$  during which it is unable to detect any photons:

$$f_{\text{recovery}}(t) = 0 \quad (3)$$

This means that in general,  $f(t)$  depends on the probability  $P(t - \tau_{\text{reset}}, t)$  that a pulse occurred less than the recovery period before the time  $t$ . Therefore, the overall expression for  $f(t)$  is a non-linear integral equation:

$$f(t) = (\eta_{\text{PDP}}\rho_{ph}(t) + R_{\text{dark}}) \left( 1 - \int_{t-\tau_{\text{reset}}}^t dt' f(t') \right) \quad (4)$$

Equation (4) is the master equation for all the following considerations.

## 3 Useful approximations and special cases

### 3.1 Photon statistics

The incoming photon stream  $\rho_{ph}(t)$  is a random distribution of individual photons with certain statistical properties. Peculiar statistical phenomena between individual photons are typically observed on timescales on the order of several ps or less. This time distribution of photons can follow a controllable envelope function which contains the data which we want to transmit. Here we are going to examine effects on a timescale larger than the recovery time  $\tau_{\text{reset}}$ . This is typically on the order of 10s of ns, but at least several ns. Therefore subtle effects like photon (anti-)bunching do not need to be considered here. We can therefore split  $\rho_{ph}$  into two components:

$$\rho_{ph}(t) = \rho_{\text{signal}}(t) + \rho_{bg} \quad (5)$$

where  $\rho_{\text{signal}}(t)$  carries the data signal and  $\rho_{bg}$  is the background, which is assumed to be constant here.

### 3.2 Static solution

If  $\rho_{\text{signal}}(t) \equiv 0$ , then  $f(t)$  is constant:

$$f(t) \equiv f_{bg} = \frac{\rho_{bg}\eta_{\text{PDP}} + R_{\text{dark}}}{1 + \tau_{\text{reset}}(\rho_{bg}\eta_{\text{PDP}} + R_{\text{dark}})} \quad (6)$$

Note that in the limit of infinitely intense light, the SPAD triggers a pulse as soon as it has recovered from the previous one, i.e. the pulse rate is given by the recovery time:

$$\lim_{\rho_{bg} \rightarrow \infty} f_{bg} = \frac{1}{\tau_{reset}} \quad (7)$$

### 3.3 Response to a short pulse

Let us assume an infinitely short pulse:

$$\rho_{signal}(t) = \rho_0 \delta(t) \quad (8)$$

where  $\rho_0$  corresponds to the pulse energy and  $\delta(t)$  is the Dirac- $\delta$ . Let us integrate  $f(t)$  over an interval  $[-t_1, t_1]$ :

$$\begin{aligned} \int_{-t_1}^{t_1} dt f(t) &= t_1 f_{bg} + \rho_0 \eta_{PDP} (1 - \tau_{reset} f_{bg}) + \\ \int_{0^+}^{t_1} dt (\rho_{bg} \eta_{PDP} + R_{dark}) \left( 1 - \int_{t-\tau_{reset}}^t dt' f(t') \right) & \quad f(t) = f_{bg} + \sum_i \delta(t_i) \rho_i \eta_{PDP} (1 - \tau_{reset} f_{bg}) \end{aligned} \quad (9)$$

From equation (9) we can readily give  $f(t)$  in the interval  $(-\infty, 0]$ :

$$f(t) = \begin{cases} f_{bg} & , t < 0 \\ \delta(t) \rho_0 \eta_{PDP} (1 - \tau_{reset} f_{bg}) & , t = 0 \\ (\rho_{bg} \eta_{PDP} + R_{dark}) \left( 1 - \int_{t-\tau_{reset}}^t dt' f(t') \right) & , t > 0 \end{cases} \quad (10)$$

#### 3.3.1 Low signal/high background approximation

If the influence of the background on the integral  $\int_{t-\tau_{reset}}^t dt' f(t')$  in equation (10) is dominant throughout, then a complete analytical expression for  $f(t)$  can be given. This is the case if:

$$\rho_0 \eta_{PDP} (1 - \tau_{reset} f_{bg}) \ll \tau_{reset} f_{bg} \quad (11)$$

In this case we have:

$$f(t) = f_{bg} + \delta(t) \rho_0 \eta_{PDP} (1 - \tau_{reset} f_{bg}) \quad (12)$$

Equation (12) will be used for all the following considerations due to its simplicity. As long as the timescales of interest are longer than  $\tau_{reset}$ , this approximation is expected to be useful even if equation (11) is not fulfilled.

#### 3.3.2 Pulse trains

Consider not just a single pulse, but a set of discrete pulses at times  $t_i$  and pulse energy  $\rho_i$ ,  $i \in \mathbb{N}$ . Then equation (12) can be rewritten to:

### 3.4 Summary

The probability  $f(t)dt$  for recording a SPAD pulse in the time interval  $[t, t + dt]$  is given by equation (13) provided that the following approximations are applicable:

- The optical signal consists of discrete pulses where each pulse is shorter than  $\tau_{reset}$
- The background illumination can be assumed constant on the timescale of the spacing between pulses.
- $\tau_{reset}$  and the spacing between pulses are both longer than the timescale at which effects like photon bunching or antibunching are visible.
- Either equation (11) is fulfilled or the timescales that are considered (in particular the spacing between pulses) are longer than  $\tau_{reset}$

## 4 Transmission protocol

Equation (13) is based on the emission of discrete short pulses. Therefore, two modulation schemes for transmitting data appear as a natural choice: pulse position modulation (PPM) and pulse amplitude modulation (PAM). Let us first consider PPM as it provides a natural way of dealing with the problem of not being able to trigger directly from the received optical signal.

### 4.1 Photon timing statistics

Let us monitor the output of the SPAD during a finite time interval  $[-t_1, t_1]$ . If we received a SPAD count at time  $t$ , what is the probability of receiving another count at time  $t + \tau$ ? Obviously, during the recovery period  $\tau_{reset}$  this probability is 0 and then within another period on the order of  $\tau_{reset}$  the probability distribution relaxes back to the undistorted  $f(t)$ . For simplicity, let us only consider timescales longer than this relaxation process:

$$\tau \gg \tau_{reset} \quad (\text{practically: } \tau > \sim 2\tau_{reset}) \quad (14)$$

Then  $f(t)dt$  is the probability of recording a count in the interval  $[t, t+dt]$  and the probability of subsequently receiving a second count in the interval  $[t+\tau, t+\tau+dt']$  is  $f(t)dt f(t+\tau)dt'$ . The total number  $N$  of recorded counts is given by integration:

$$N = \int_{-t_1}^{t_1} dt f(t) \quad (15)$$

Similarly, the number of counts  $N'$  that were received within a time separation interval  $[\tau, \tau+\Delta t']$  after an initial count is also given by integration:

$$N' = \int_{\tau}^{\tau+\Delta t'} dt' \int_{-t_1}^{t_1} dt f(t)f(t+t') \quad (16)$$

Therefore, the count density function  $g(\tau)dt'$  of recording two subsequent SPAD counts with temporal separation in the interval  $[\tau, \tau+dt']$  is:

$$g(\tau) = \int_{-t_1}^{t_1} dt f(t)f(t+\tau) \quad (17)$$

Note that equation (17) only relies on one single approximation, namely equation (14). For a periodically repeated signal,  $g(\tau)$  can directly be obtained from the output of a single SPAD, i.e. *data can be received by measuring  $g(\tau)$* .

### 4.2 PPM

Let us assume two subsequent pulses at times  $t = 0$  and  $t = T$  with pulse energies  $\rho_0$  and  $\rho_P$ , see also Fig. 1 below:

$$\begin{aligned} \rho_{signal}(t) &= \rho_0\delta(t) + \rho_P\delta(t-T) \\ f(t) &= f_{bg} + \delta(t)\rho_0\eta_{PDP}(1 - \tau_{reset}f_{bg}) \\ &\quad + \delta(t-T)\rho_P\eta_{PDP}(1 - \tau_{reset}f_{bg}) \end{aligned} \quad (18)$$

In this case, equation (17) becomes (taking advantage of the fact that  $\tau > 0$  strictly):

$$\begin{aligned} g(\tau) &= 2t_1 f_{bg}^2 + 2f_{bg}\eta_{PDP}(1 - \tau_{reset}f_{bg})(\rho_0 + \rho_P) \\ &\quad + \delta(\tau - T)\rho_0\rho_P\eta_{PDP}^2(1 - \tau_{reset}f_{bg})^2 \end{aligned} \quad (19)$$

We observe that *the separation  $T$  between the pulses is marked by a peak in  $g(\tau)$  at  $\tau = T$* . This allows straight-forward implementation of PPM on both transmitter and receiver end. Note that the high timing accuracy of SPADs could in principle allow very high modulation orders.

In the simplest case, a single pulse position can be used, and data encoded in the presence or absence of this pulse. In this case, the transmission resembles on-off keying (OOK). This encoding method was used in the work discussed in the main article to demonstrate the feasibility of the transmission method, due to its simplicity. Analytical investigations into potential data rates showed only minor improvements in data rate using more complex PPM over OOK transmission. It is possible that using a SPAD and/or transmitter with different parameters may improve the potential gain of PPM transmission.

### 4.3 PAM

In equations (18) and (19), the amplitude  $\rho_P$  of the second pulse can in principle assume any number of discrete levels, thus enabling PAM. However, gauging of the intensity levels needs to be done. This could be done via a training sequence. In the case of a periodically repeated signal such as shown in Fig. 1, the gauging can also be obtained via comparison of  $g(T)$  and  $g(\tau_{rep})$ , which in principle allows retrieval of the ratio between  $\rho_0$  and  $\rho_P$ . Fig. 1 also shows that PAM and PPM can easily be combined.

### 4.4 Implementation

In reality, in order to allow sufficient sampling, the signal needs to be repeated periodically with a period  $\tau_{rep}$ :

$$\rho_{signal} = \sum_{n=-\infty}^{\infty} [\rho_0(t - n\tau_{rep}) + \rho_P(t - n\tau_{rep} - T)] \quad (20)$$

The receiver samples SPAD counts over a sampling period  $T_s$  into time bins  $t_i$ ,  $i = 1, \dots, N_S$ ,

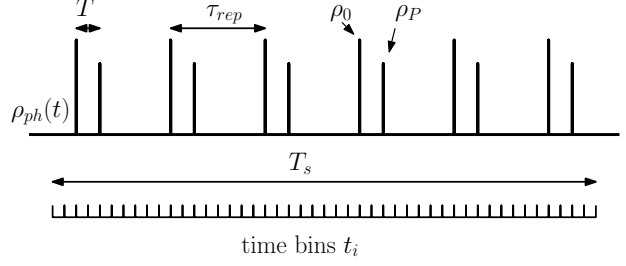

Figure 1: Illustration of the proposed transmission protocol. Two successive pulses with temporal separation  $T$  and amplitudes  $\rho_0$  and  $\rho_P$  are transmitted periodically with repetition period  $\tau_{rep}$ . The receiver samples photon counts over a sampling time  $T_s$  into time bins  $t_i$ .

where  $N_s$  is the number of samples. This scheme is illustrated in Fig. 1. The time bins have a size  $t_{bin} = t_{i+1} - t_i$ . After sampling, each time bin  $t_i$  contains a number of counts  $f_i$ . If the time bin size is chosen smaller than the SPAD recovery time  $t_{bin} < \tau_{reset}$ , then  $f_i \in \{0, 1\}$  is binary, thus simplifying the numerical effort for calculating  $g(\tau)$ .

#### 4.4.1 Calculation of $g(\tau)$

The correlation time  $\tau$  is also discretised into correlation time bins  $\tau_j$ ,  $j = 1, \dots, N_\tau$ . It is sensible to choose the correlation time bin size  $\tau_{bin} = \tau_{j+1} - \tau_j$  as an integer multiple of the sampling bin size  $\tau_{bin} = k t_{bin}$ ,  $k \in \mathbb{N}^+$ . It is useful to define start and stop indices  $n_{start}$  and  $n_{stop}$ :

$$n_{start} = \frac{\tau_1}{t_{bin}} \quad (21)$$

$$n_{stop} = n_{start} + k N_\tau - 1 \quad (22)$$

Then the discretised version of equation (17) can be written as:

$$g(\tau_j) = \sum_{i=1}^{N_s - n_{stop}} \sum_{l=0}^{k-1} f_i f_{i+n_{start}+(j-1)k+l} \quad (23)$$

in the case when  $t_{bin} < \tau_{reset}$  and thus  $f_i$  is binary, the multiplication in equation (23) can be replaced by **if**-statements and the summation can be done by counters, i.e. the calculation of  $g(\tau)$  can be implemented with simple standard logic circuits.

## 5 Embedded clock

Due to the probabilistic nature of the SPAD signal, edge-detection is not easily available to facilitate clock synchronisation (but could be made available via over-sampling). Here we discuss an anisochronous embedded clock to be specifically used with OOK encoding which will allow to keep the sampling rate the same as the symbol rate.

### 5.1 Frame-level synchronisation

The embedded clock can be realised by a “magic clock word” of  $n_{clk}$  bits length which is sent at the start of each frame with length  $N_{frame} = n_{clk} + n_{dat}$ , where  $n_{dat}$  is the number of data bits per frame. This structure is illustrated in figure 2. Let us assume that we use  $M$  frames for the frame-level clock-synchronisation procedure. Then we want to know the probability  $P_{err}$  that the clock is erroneously synchronised to a randomly occurring replica of the magic clock word sequence in the data stream. In the case of error free transmission (BER=0),  $P_{err}$  can readily be calculated as:

$$P_{err}(n_{clk}, n_{dat}, M) = \frac{p(n_{clk}, n_{dat}, M)}{1 + p(n_{clk}, n_{dat}, M)} \quad (24)$$

Where  $p(n_{clk}, n_{dat}, M)$  is the average number of false clock word sequences in the data stream. It can be calculated recursively:

$$p(n_{clk}, n_{dat} < n_{clk}, M) = 0 \quad (25a)$$

$$p(n_{clk}, n_{dat} = n_{clk}, M) = \frac{1}{2^{n_{clk}M}} \quad (25b)$$

$$\begin{aligned} p(n_{clk}, n_{dat} > n_{clk}, M) &= \frac{1}{2^{n_{clk}M}} (1 + p(n_{clk}, n_{dat} - n_{clk}, M)) \\ &+ \left(1 - \frac{1}{2^{n_{clk}M}}\right) p(n_{clk}, n_{dat} - 1, M) \end{aligned} \quad (25c)$$

Note that all three equations, but in particular (25a) are valid for BER=0 on the one hand, but on the other hand also require clever choice of the magic clock word. Namely, the clock word has to be chosen such that part of the clock word cannot be completed to a replica of the clock word by adding matching data bits in the data word before/after the clock word. An unwise choice (e.g. “010101”) would yield a larger  $p(n_{clk}, n_{dat}, M)$  than calculated in equation (25).

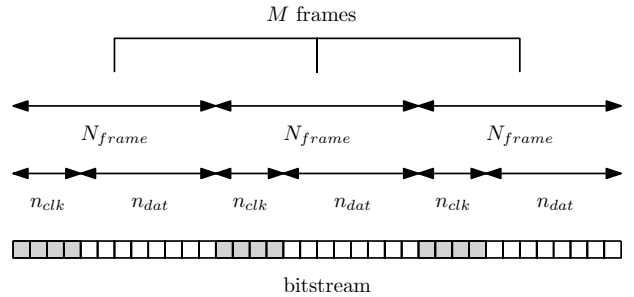

Figure 2: Schematic illustration of the division of the bitstream into frames, which in turn consist of a clock word of  $n_{clk}$  bits followed by a data word of  $n_{dat}$  bits.  $M$  such frames are used for frame-level synchronisation.

The frame-level synchronisation variables

$n_{clk}, n_{dat}, M$  should practically be chosen such that  $P_{err}$  calculated by equations (24) and (25) matches the target BER of the system. Within this constraint and possible other constraints not considered here, it will be useful to try to find an application-specific trade-off between minimising  $M \cdot N_{frame}$  for quick clock synchronisation and maximising  $n_{dat}/n_{clk}$  for high data throughput. Below in section 5.2 a clock word length of  $n_{clk} = 6$  is suggested. Based on this we can, for example, choose:

$$n_{clk} = 6 \quad (26a)$$

$$n_{dat} = 32 \quad (26b)$$

$$M = 6 \quad (26c)$$

$$P_{err} = 3.9 \times 10^{-10} \quad (26d)$$

This allows frame-level synchronisation on the basis of 228 transmitted bits.

## 5.2 Symbol-level synchronisation

Consider the 6-bit clock word “001101”. It has properties that are useful for frame-level synchronisation as discussed in section 5.1. However, while frame-level synchronisation allows to distinguish between data bits and clock signal bits, an additional mechanism for symbol-level phase synchronisation between the transmitter and receiver clocks is needed. In this section, it is discussed how the above clock word can enable symbol-level synchronisation when the receiver sampling rate is the same as the symbol rate.

Figure 3 illustrates how symbol-level synchronisation is achieved. Let  $r_x(t)$  be the received correlation counts at receiver time-frame  $t$ . Let  $r_x^{(1)}$  be the correlation counts corresponding to a transmitted “1” under perfect clock synchronisation and  $r_x^{(0)}$  the correlation counts corresponding

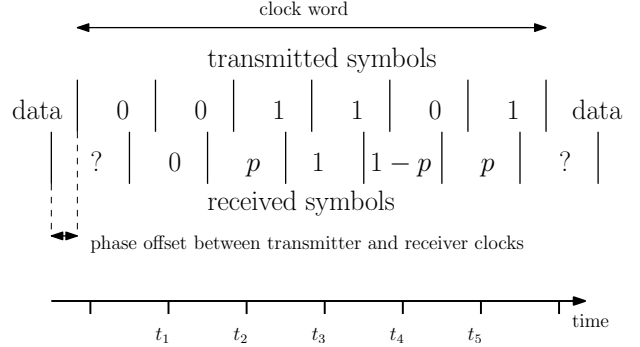

Figure 3: Schematic illustration of symbol-level synchronisation. The transmitted and received symbols are sampled with a phase offset which needs to be determined and subsequently corrected.

to a “0”. Then the received correlation counts at the 5 time frames  $t_1, \dots, t_5$  indicated in figure 3 are:

$$r_x(t_1) = r_x^{(0)} \quad (27a)$$

$$r_x(t_2) = p \cdot r_x^{(1)} + (1 - p)r_x^{(0)} \quad (27b)$$

$$r_x(t_3) = r_x^{(1)} \quad (27c)$$

$$r_x(t_4) = (1 - p)r_x^{(1)} + p \cdot r_x^{(0)} \quad (27d)$$

$$r_x(t_5) = p \cdot r_x^{(1)} + (1 - p)r_x^{(0)} \quad (27e)$$

$$p \in [0, 1] \quad (27f)$$

Here,  $p$  is a parameter that is directly related to the phase offset between the two clocks. If  $p = 0$ , then the clocks are perfectly synchronised, and otherwise it can be used to determine by how much the receiver phase needs to be corrected to achieve synchronisation. Note that this pattern allows not only clock synchronisation, but also determination of the correlation count levels for 0 and 1 and thus the threshold for OOK decoding.

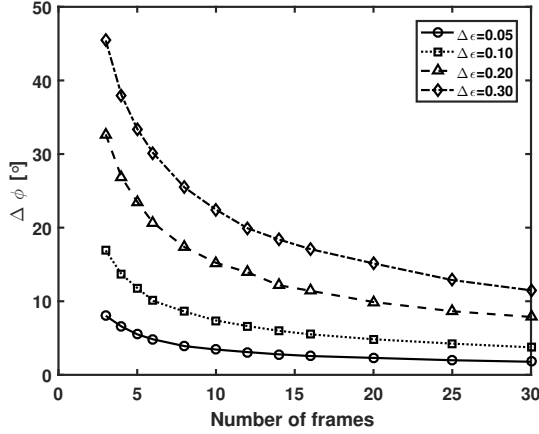

Figure 4: Simulated performance of symbol-level synchronisation: precision of phase shift measurement as a function of the number of received frames.

Due to the variability in the receiver counts, it is advisable to use more than one repeat of the clock word to measure  $p$ ,  $r_x^{(1)}$  and  $r_x^{(0)}$ . This has been investigated with a simulation, where a random bit sequence was interleaved with the above clock word, noise was added and the stream was sampled at phase shifts  $\varphi$  between  $-90^\circ$  and  $-90^\circ$ . Performing symbol-level synchronisation on this sampled stream yields a measured phase shift  $\phi$ . The standard deviation  $\Delta\phi$  of this measurement was taken from 1000 samples for each given  $\varphi$ . In figure 4,  $\Delta\phi$  is plotted as a function of the number of frames used for synchronisation for several noise scenarios. In order to resemble experimental observations, Gaussian noise  $\epsilon$  with a standard deviation of  $\Delta\epsilon$  was added to the “1” symbols, but not to the “0” symbols in the transmitted stream:

$$\begin{aligned} r_x^{(1)} &= (1 + \epsilon) \\ r_x^{(0)} &= 0 \end{aligned} \quad (28)$$

Equation (28) gives a good resemblance of the signal extracted from oscilloscope traces in a dark to moderately lit environment. At  $\Delta\epsilon = 0.3$  the trace appears similar to those with a BER between  $10^{-3}$  and  $10^{-4}$ .

Figure 4 suggests that if a desired precision of  $15^\circ$  in the phase measurement is desired, then 25 frames should be used. This in turn means (at  $N_{frame} = 38$ ) that the clock frequencies of transmitter and receiver should have a precision of  $\sim 90$  ppm to ensure reliable operation. This requirement can be loosened by using a longer clock word if needed.

### 5.2.1 Generalisation of the clock word

Clock words  $w_{clk}$  with the same properties as the 6-bit word used here but different lengths can be constructed from elementary building blocks  $B_n$ :

$$\begin{aligned} B_n &= \overbrace{00 \dots 0}^n \overbrace{11 \dots 1}^n \\ w_{clk} &= B_{n(1)} B_{n(2)} \dots B_{n(m)} \\ n^{(i)} &\neq n^{(j)} \quad \forall i \neq j \end{aligned} \quad (29)$$

The resulting clock word has a length of  $2 \sum_{i=1}^m n^{(i)}$  bits and its inverse is also a possible clock word.

### 5.2.2 OOK threshold

If several clock word repetitions are used to determine  $r_x^{(1)}$  and  $r_x^{(0)}$ , then their variances  $\Delta^{(1)}$  and  $\Delta^{(0)}$  can be measured at the same time. With the knowledge of these variables, a sensible setting

for the OOK threshold  $r_{OOK}$  that discriminates whether a given  $r_x(t)$  is a “1” or “0” is given by:

$$r_{OOK} = \frac{1}{2} \left( r_x^{(1)} - \Delta^{(1)} + r_x^{(0)} + \Delta^{(0)} \right) \quad (30)$$

This allows continuous adaptation (performed at during each symbol-level synchronisation) of the OOK threshold to a temporally varying level of background counts.

### 5.3 Simultaneous frame- and symbol-level synchronisation in the initial step

The frame-level synchronisation described in section 5.1 assumes that symbol-level synchronisation is perfect, and in turn, the symbol-level synchronisation describe in section 5.2 requires knowledge of the temporal position of the clock word, *i.e.* frame-level synchronisation. At the start of operation, neither is given and therefore both have to be achieved at the same time. This can be done by searching for periodic occurrence of the 5-symbol pattern given in equation (27) in the stream of received counts, with a period of  $N_{frame}$ .

The performance of the method was investigated in a similar way as described in section 5.2 for phase shifts  $\varphi$  over the entire possible range from  $-180^\circ$  to  $-180^\circ$ . A result in a high noise scenario is shown in figure 5. It can be seen by comparison to figure 4 that the performance is essentially limited by the symbol-level synchronisation and therefore the same number of frames should be used.

At any later time, whenever the phase offset, measured by  $p$ , is found to be excessively large, then this can be taken as an indication

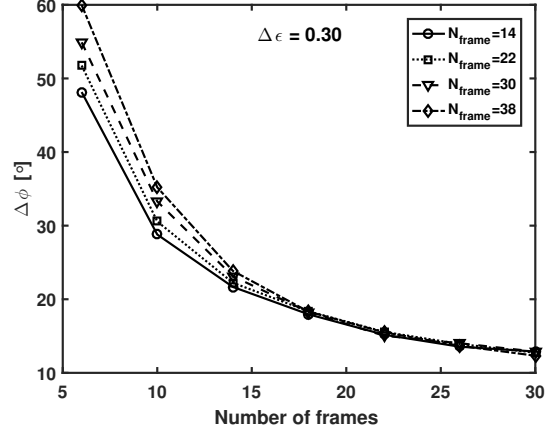

Figure 5: Simulated performance of simultaneous frame- and symbol-level synchronisation: precision of phase shift measurement as a function of the number of received frames.

that both symbol- and frame-level synchronisation have been lost and the above process can be triggered to re-establish synchronisation.

## 6 Power measurement under DC illumination

Consider a SPAD with photon detection probability  $\eta_{PDP}$ , dark count rate  $R_{dark}$  and dead time  $\tau_{dead}$ . Given an incident photon flux  $\Phi(t)$ , then the probability  $P(t)dt$  of receiving a SPAD count in the time interval  $[t, t + dt]$  is:

$$P(t)dt = (\eta_{PDP}\Phi(t) + R_{dark})(1 - P_{dead}(t))dt \quad (31)$$

where  $P_{dead}(t)$  is the probability that at time  $t$  the SPAD is still undergoing a recovery cycle from a previous photon count. It is given by

Eq. (32):

$$P_{dead}(t) = \int_{t-\tau_{dead}}^t dt' P(t') \quad (32)$$

Eqs. (31) and (32) form a set of integral equations that may be difficult to solve. However, in steady state ( $\Phi(t) \equiv \Phi_{DC}$ ) we have  $P_{DC} = R_{DC}$ , where  $R_{DC}$  is the detector count rate and we can readily solve for the incident photon flux  $\Phi_{DC}$ :

$$\Phi_{DC} = \frac{1}{\eta_{PDP}} \left( \frac{R_{DC}}{1 - \tau_{dead} R_{DC}} - R_{dark} \right) \quad (33)$$

The incident optical DC power is then given by:

$$P_{DC} = \frac{hc}{\lambda} \Phi_{DC} \quad (34)$$

where  $h$  is the Planck constant,  $c$  the speed of light and  $\lambda$  is the wavelength of the source.

## 7 Power measurements under pulsed conditions

Under the pulsed conditions used for the low light level encoding discussed in the main text, the integral Eqs. (31) and (32) can also be replaced by a simplified approach.

Assume that the incident light on a SPAD is a continuous series of short optical pulses at a constant repetition rate  $R_{rep}$ . If the individual pulses are shorter than the SPAD dead time, and the pulse separation  $\tau_{rep} = 1/R_{rep}$  is longer than the SPAD dead time, then the average incident optical power and the average number of incident photons per pulse can be calculated as detailed below.

For one optical pulse, we get at most one SPAD count because the SPAD dead time is longer than the pulse duration. Let us assume a single pulse

with  $n \in \mathbb{N}$  photons. Then the probability  $P_{count}^{(n)}$  of receiving one photon count from this pulse is:

$$P_{count}^{(n)} = \sum_{i=1}^n \eta_{PDP} (1 - \eta_{PDP})^{i-1} \quad (35)$$

where  $\eta_{PDP}$  is the photon detection probability of the SPAD. Note that equation (35) uses the identities  $\sum_{i=1}^0 \equiv 0$  and  $\prod_{j=1}^0 \equiv 1$ .

Therefore, the probability  $P_{count}$  of receiving a photon count for any pulse is:

$$P_{count}(n_{av}) = \sum_{n=0}^{\infty} P_{n_{av}}(n) \cdot P_{count}^{(n)} \quad (36)$$

where  $P_{n_{av}}(n)$  is the probability that a given pulse has  $n$  photons incident on the SPAD.  $P_{n_{av}}(n)$  follows a Poisson distribution with average photon number  $n_{av} \in \mathbb{R}^+$ :

$$P_{n_{av}}(n) = \frac{n_{av}^n}{n!} e^{-n_{av}} \quad (37)$$

On the other hand,  $P_{count}$  can be obtained experimentally from the measured signal count rate  $R^{(1)}$  (the superscript  $(1)$  indicates that this measurement corresponds to transmission of a constant binary value 1):

$$P_{count,exp} \approx \frac{R^{(1)} - R_{dark}}{R_{rep}} \quad (38)$$

where  $R_{dark}$  is the dark count rate of the detector.

We can then determine  $n_{av}$  by numerically solving for:

$$P_{count}(n_{av}) - P_{count,exp} = 0 \quad (39)$$

The average incident photon flux  $\Phi_{inc}^{(1)}$  is then:

$$\Phi_{inc}^{(1)} = R_{rep} n_{av} \quad (40)$$

The incident power  $P_{inc}^{(1)}$  is then given by:

$$P_{inc}^{(1)} = \frac{hc}{\lambda} \Phi_{inc}^{(1)} \quad (41)$$

## 7.1 Incident power during data transmission

Note that the LED operation for this measurement corresponds to transmission of a constant value of 1. For data transmission, the average incident power is thus taken as half the value obtained by the method above, as for a value of 0 the incident optical power is 0.

$$\Phi_{inc} = \Phi_{inc}^{(1)}/2 \quad (42)$$

$$P_{inc} = P_{inc}^{(1)}/2 \quad (43)$$

Where  $\Phi_{inc}$  is the average incident photon flux of the data signal under the absence of background illumination and  $P_{inc}$  the average incident power.

## 7.2 Measuring photons per bit

Note that  $n_{av}$  is the average number of photons per pulse that are incident on the detector. Given the data rate  $R_{data}$ , the number of incident photons per bit  $n_{inc}$  is given by Eq. (44)

$$n_{inc} = \frac{n_{av}R_{rep}}{2R_{data}} \quad (44)$$

The factor 2 in Eq. (44) again accounts for the fact that pulses are only present upon transmission of a binary 1 and absent during transmission of a 0. Pay careful attention to the fact that  $n_{inc}$  is different from the received number of photons per bit  $n_{rec}$ :

$$n_{rec} \approx \frac{R_{sig}^{(1)} - R_{dark}}{2R_{data}} \quad (45)$$

The standard quantum limit applies to  $n_{rec}$ , which is in good approximation related to  $n_{inc}$  via Eq. (46)

$$n_{rec} \approx \eta PDP n_{inc} \quad (46)$$

## 8 Summary

- Data can be received with a single SPAD by measuring the self-correlation  $g(\tau)$  of the SPAD output as given by equation (17).
  - In practice,  $g(\tau)$  can be calculated using equation (23).
- PPM and PAM are enabled based on transmission and decoding via equations (18) and (19). PPM is believed to be easier to implement than PAM. Both can readily be combined.
  - A periodical signal as given in equation (20) should be used in practice.
  - Both PPM and PAM should in principle not need any training sequences.
  - A visual illustration of the transmitted signal and its sampling is given in Fig. 1.
  - Encouraging experimental results were obtained using OOK.
- An embedded clock for OOK transmission has been suggested that allows frame- and symbol-level clock synchronisation.
  - A 6-bit clock word is discussed in detail, but generalisation to other clock word lengths has been outlined.
  - It is suggested to use 25 received frames for symbol-level synchronisation.
  - It is suggested to use 6 received frames for frame-level synchronisation.
- Received optical power can be calculated from the received photon count rate using numerical methods.

Table 1: Table of modulated background conditions for results in Figure 3d) in the main article. Optical power of the modulated background interference, signal power and histogram threshold are shown.

| Curve | Background<br>Data Rate | $P_{bg}$<br>( $pW$ ) | $P_s$<br>( $pW$ ) | Threshold<br>( <i>counts</i> ) |
|-------|-------------------------|----------------------|-------------------|--------------------------------|
| a     | DC                      | 15.01                | 9.9               | 25                             |
| b     | 10 kHz                  | 16.22                | 13.9              | 39                             |
| c     | 40 kHz                  | 15.54                | 13.4              | 39                             |
| d     | 50 kHz                  | 15.08                | 13.2              | 37                             |
| e     | 62.5 kHz                | 15.15                | 13.3              | 37                             |
| f     | 100 kHz                 | 15.01                | 13.4              | 37                             |
| g     | 1 MHz                   | 15.04                | 10.7              | 27                             |
| h     | 10 MHz                  | 15.18                | 10                | 24                             |

Table 2: Table of signal conditions required to obtain a BER of  $10^{-3}$  for results in Figure 3d) in the main article.

| Curve | Detector Count<br>Rate ( $s^{-1}$ ) | Incident Photon<br>Flux ( $ph/s$ ) | Optical Power<br>( $pW$ ) | Threshold<br>( <i>counts</i> ) |
|-------|-------------------------------------|------------------------------------|---------------------------|--------------------------------|
| a     | $3.60 \times 10^6$                  | $2.02 \times 10^7$                 | 9.9                       | 25                             |
| b     | $4.74 \times 10^6$                  | $2.83 \times 10^7$                 | 13.9                      | 39                             |
| c     | $4.60 \times 10^6$                  | $2.73 \times 10^7$                 | 13.4                      | 39                             |
| d     | $4.55 \times 10^6$                  | $2.69 \times 10^7$                 | 13.2                      | 37                             |
| e     | $4.57 \times 10^6$                  | $2.71 \times 10^7$                 | 13.3                      | 37                             |
| f     | $4.60 \times 10^6$                  | $2.73 \times 10^7$                 | 13.4                      | 37                             |
| g     | $3.84 \times 10^6$                  | $2.18 \times 10^7$                 | 10.7                      | 27                             |
| h     | $3.63 \times 10^6$                  | $2.04 \times 10^7$                 | 10                        | 24                             |

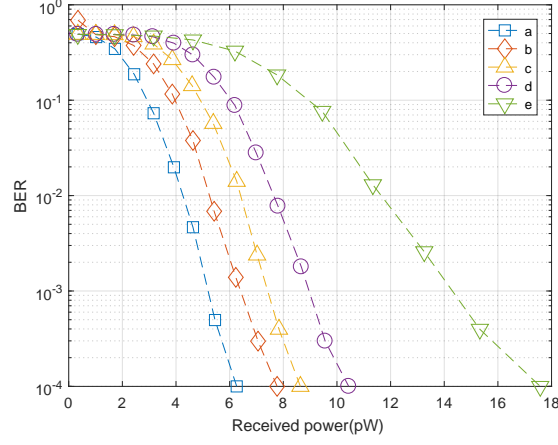

Figure 6: BER curves for constant background conditions. Conditions for curves a-e can be found in Table 1 in the main article.

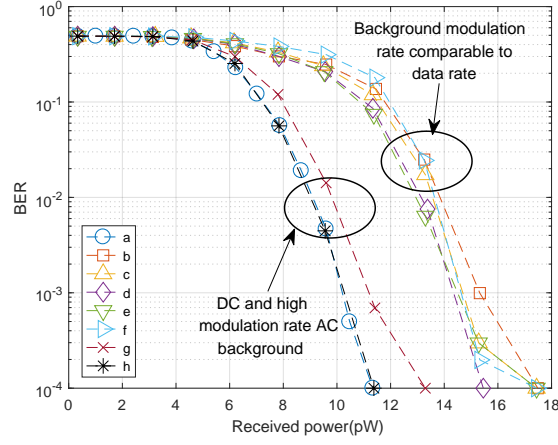

Figure 7: BER curves for modulated background conditions. Conditions for curves a-h can be found in Tables 1 and 2.
